# Supplementary material for: Lossy Compression for Lossless Prediction
Source: arXiv:2106.10800 source file (2022-01-28)
Supplement: Supplementary file 1 [file checklist.tex]

\begin{enumerate}

\item For all authors...
\begin{enumerate}
  \item Do the main claims made in the abstract and introduction accurately reflect the paper's contributions and scope?
    \answerYes{}
  \item Did you describe the limitations of your work?
    \answerYes{In \cref{sec:conclusion}.}
  \item Did you discuss any potential negative societal impacts of your work?
    \answerYes{In \cref{sec:conclusion} we mention the potential decrease in interpretability. }
  \item Have you read the ethics review guidelines and ensured that your paper conforms to them?
    \answerYes{}
\end{enumerate}

\item If you are including theoretical results...
\begin{enumerate}
  \item Did you state the full set of assumptions of all theoretical results?
    \answerYes{See \cref{appx:assumptions}.}
	\item Did you include complete proofs of all theoretical results?
    \answerYes{See \cref{appx:proofs}. }
\end{enumerate}

\item If you ran experiments...
\begin{enumerate}
  \item Did you include the code, data, and instructions needed to reproduce the main experimental results (either in the supplemental material or as a URL)?
    \answerYes{The code to train our main compressor is in \cref{appx:code_clip}, the code to replicate all our results is at \url{anonymous}.}
  \item Did you specify all the training details (e.g., data splits, hyperparameters, how they were chosen)?
    \answerYes{The most important training details can be found at \cref{appx:reproducability}. Minor hyperparameters can be found in our code at  \url{anonymous}. }
	\item Did you report error bars (e.g., with respect to the random seed after running experiments multiple times)?
    \answerYes{We report error bars for MNIST (\cref{appx:mnist}) and Banana (\cref{appx:banana}). For larger experiments we sampled a fixed number of hyperparameters for each model and baseline (see \cref{appx:reproducability}), and report the best result.
    }
	\item Did you include the total amount of compute and the type of resources used (e.g., type of GPUs, internal cluster, or cloud provider)?
    \answerNo{}
\end{enumerate}

\item If you are using existing assets (e.g., code, data, models) or curating/releasing new assets...
\begin{enumerate}
  \item If your work uses existing assets, did you cite the creators?
    \answerYes{In \cref{appx:reproducability}.}
  \item Did you mention the license of the assets?
    \answerNo{} 
  \item Did you include any new assets either in the supplemental material or as a URL?
    \answerYes{Our clip compressor in \cref{appx:code_clip} and our code at \url{anonymous}.}
  \item Did you discuss whether and how consent was obtained from people whose data you're using/curating?
    \answerNo{We do not propose any new dataset. The main possible issues come from the CLIP dataset \cite{radford_learning_2021}, for which the data collection procedure is discussed in details in their paper.
    }
  \item Did you discuss whether the data you are using/curating contains personally identifiable information or offensive content?
  \answerNo{We do not propose any new dataset.  The main possible issues come from the CLIP dataset \cite{radford_learning_2021}, for which the data collection procedure is discussed in details in their paper.
  }
\end{enumerate}

\end{enumerate}
